# Supplementary material for: Towards a Client-Centered Assessment of LLM Therapists by Client Simulation
Source: arXiv:2406.12266 source file (2024-06-20)
Supplement: Supplementary file 1 [file appendix.tex]

\paragraph{Beck Depression Inventory (BDI)}
The BDI is a self-report rating inventory that measures characteristic attitudes and symptoms of depression \cite{beck1961inventory}. It consists of $21$ questions about how the patient has been feeling in the last week. When the test is scored, a value of $0$ to $3$ is assigned for each answer, and then the total score is compared to a key to determine the severity of the depression. Therefore, BDI sum scores range from $0$ to $63$, with scores of $\geq11$, $\geq17$, $\geq21$, $\geq31$, and $\geq41$ representing mild mood and disturbance, borderline clinical depression, moderate depression, severe depression, and extreme depression. The items of BDI are displayed in \Cref{tab:appendix:BDI}.
\begin{table*}[tbh]
    \footnotesize
    \centering
    \begin{tabular}{m{.0275\textwidth}<{\centering}m{.425\textwidth}|m{.0275\textwidth}<{\centering}m{.425\textwidth}}
    \hline
    \textbf{No} & \textbf{Score \& BDI Item} & \textbf{No} & \textbf{Score \& BDI Item} \\
    \hline
    \multirow{4}{*}{1} & 0~~I do not feel sad. & \multirow{4}{*}{12} & 0~~I have not lost interest in other people. \\
        & 1~~I feel sad. &  & 1~~I am less interested in other people than I used to be. \\
        & 2~~I am sad all the time and I can't snap out of it. &  & 2~~I have lost most of my interest in other people. \\
        & 3~~I am so sad and unhappy that I can't stand it. &  & 3~~I have lost all of my interest in other people. \\
    \hline
    \multirow{6}{*}{2} & 0~~I am not particularly discouraged about the future. & \multirow{6}{*}{13} & 0~~I make decisions about as well as I ever could.\\
        & 1~~I feel discouraged about the future.  &  & 1~~I put off making decisions more than I used to. \\
        & 2~~I feel I have nothing to look forward to.  &  & 2~~I have greater difficulty in making decisions more than I used to. \\
        & 3~~I feel the future is hopeless and that things cannot improve. &  & 3~~I can't make decisions at all anymore. \\
    \hline
    \multirow{5}{*}{3} & 0~~I do not feel like a failure.  & \multirow{5}{*}{14} & 0~~I don't feel that I look any worse than I used to. \\
        & 1~~I feel I have failed more than the average person.  &  & 1~~I am worried that I am looking old or unattractive. \\
        & 2~~As I look back on my life, all I can see is a lot of failures.  &  & 2~~I feel there are permanent changes in my appearance that make me look unattractive. \\
        & 3~~I feel I am a complete failure as a person.  &  & 3~~I believe that I look ugly. \\
    \hline
    \multirow{5}{*}{4} & 0~~I get as much satisfaction out of things as I used to.  & \multirow{5}{*}{15} & 0~~I can work about as well as before.\\
        & 1~~I don't enjoy things the way I used to. &  & 1~~It takes an extra effort to get started at doing something.\\
        & 2~~I don't get real satisfaction out of anything anymore.  &  & 2~~I have to push myself very hard to do anything.\\
        & 3~~I am dissatisfied or bored with everything.  &  & 3~~I can't do any work at all. \\
    \hline
    \multirow{6}{*}{5} & 0~~I don't feel particularly guilty. & \multirow{6}{*}{16} & 0~~I can sleep as well as usual. \\
        & 1~~I feel guilty a good part of the time.  &  & 1~~I don't sleep as well as I used to.\\
        & 2~~I feel quite guilty most of the time.  &  & 2~~I wake up 1-2 hours earlier than usual and find it hard to get back to sleep. \\
        & 3~~I feel guilty all of the time.  &  & 3~~I wake up several hours earlier than I used to and cannot get back to sleep. \\
    \hline
    \multirow{4}{*}{6} & 0~~I don't feel I am being punished.  & \multirow{4}{*}{17} & 0~~I don't get more tired than usual.\\
        & 1~~I feel I may be punished.  &  & 1~~I get tired more easily than I used to.\\
        & 2~~I expect to be punished.  &  & 2~~I get tired from doing almost anything.\\
        & 3~~I feel I am being punished.  &  & 3~~I am too tired to do anything.\\
    \hline
    \multirow{4}{*}{7} & 0~~I don't feel disappointed in myself. & \multirow{4}{*}{18} & 0~~My appetite is no worse than usual. \\
        & 1~~I am disappointed in myself. &  & 1~~My appetite is not as good as it used to be. \\
        & 2~~I am disgusted with myself. &  & 2~~My appetite is much worse now. \\
        & 3~~I hate myself. &  & 3~~I have no appetite at all anymore. \\
    \hline
    \multirow{5}{*}{8} & 0~~I don't feel I am any worse than anybody else. & \multirow{5}{*}{19} & 0~~I haven't lost much weight, if any, lately. \\
        & 1~~I am critical of myself for my weaknesses or mistakes. &  & 1~~I have lost more than five pounds. \\
        & 2~~I blame myself all the time for my faults. &  & 2~~I have lost more than ten pounds. \\
        & 3~~I blame myself for everything bad that happens.  &  & 3~~I have lost more than fifteen pounds. \\
    \hline
    \multirow{7}{*}{9} & 0~~I don't have any thoughts of killing myself. & \multirow{7}{*}{20} & 0~~I am no more worried about my health than usual. \\
        & 1~~I have thoughts of killing myself, but I would not carry them out. &  & 1~~I am worried about physical problems like aches, pains, upset stomach, or constipation. \\
        & 2~~I would like to kill myself. &  & 2~~I am very worried about physical problems and it's hard to think of much else. \\
        & 3~~I would kill myself if I had the chance. &  & 3~~I am so worried about my physical problems that I cannot think of anything else. \\
    \hline
    \multirow{6}{*}{10} & 0~~I don't cry any more than usual. & \multirow{6}{*}{21} & 0~~I have not noticed any recent change in my interest in sex. \\
        & 1~~I cry more now than I used to. &  & 1~~I am less interested in sex than I used to be. \\
        & 2~~I cry all the time now. &  & 2~~I have almost no interest in sex. \\
        & 3~~I used to be able to cry, but now I can't cry even though I want to.  &  & 3~~I have lost interest in sex completely. \\
    \hline
    \multirow{5}{*}{11} & 0~~I am no more irritated by things than I ever was. &  &  \\
        & 1~~I am slightly more irritated now than usual. &  &  \\
        & 2~~I am quite annoyed or irritated a good deal of the time. &  &  \\
        & 3~~I feel irritated all the time.  &  &  \\
    \hline
    \end{tabular}
    \caption{Characteristics of the BDI items.}
    \label{tab:appendix:BDI}
\end{table*}

\paragraph{Outcome Rating Scale (ORS)}
The ORS \cite{miller2003outcome} is a simple, four-item measure designed to assess areas of life functioning known to change. These areas include personal or symptom distress (measuring individual well-being), interpersonal well-being (measuring how well the user is getting along in intimate relationships), social role (measuring satisfaction with work/school and relationships outside of home), and overall well-being. The ORS translates these four dimensions of functioning into four visual analog scales, which are $10$cm lines, with instructions to place a mark on each line with a low estimate to the left and a high to the right. 
\begin{figure}[tb!]
\centering
\includegraphics[width=\linewidth]{figures/Outcome-Rating-Scale.pdf} 
\caption{ORS content.}
\label{fig:appendix:ors}
\end{figure}

\paragraph{State-Trait Anxiety Inventory (STAI)}
The STAI is a validated 20-item self-report assessment that includes separate measures of state and trait anxiety \cite{spielberger1971state}. It is recommended for studying anxiety in research and clinical settings. Each of the 20 items in the STAI can be scored as $1$ (not at all), $2$ (a little), $3$ (somewhat), or $4$ (very much so). The STAI sum scores range from $20$ to $80$. The scores are commonly classified as ``no or low anxiety'' ($20\sim37$), ``moderate anxiety'' ($38\sim44$), and ``high anxiety'' ($45\sim80$). \Cref{tab:appendix:STAI} presents the content of STAI.
\begin{table}[tbh]
    \small
    
    \centering
    \begin{tabular}{m{.039\linewidth}m{.388\linewidth}|m{.039\linewidth}m{.315\linewidth}}
    \hline
    \textbf{No} & \textbf{STAI Item} & \textbf{No} & \textbf{STAI Item} \\
    \hline
    1 & I feel calm & 11 & I feel self-confident \\
    2 & I feel secure & 12 & I feel nervous \\
    3 & I feel tense & 13 & I feel jittery \\
    4 & I feel strained & 14 & I feel indecisive \\
    5 & I feel at ease & 15 & I am relaxed \\
    6 & I feel upset & 16 & I feel content\\
    7 & I am presently worrying over possible misfortunes & 17 & I am worried\\
    8 & I feel satisfied & 18 & I feel confused \\
    9 & I feel frightened & 19 & I feel steady \\
    10 & I feel uncomfortable & 20 & I feel pleasant \\
    \hline
    \end{tabular}
    \caption{Characteristics of the STAI items. Each question starts with ``\textit{Read each statement and select the appropriate response to indicate how you feel right now, that is, at this very moment. There are no right or wrong answers. Do not spend too much time on any one statement but give the answer which seems to describe your present feelings best.}''}
    \label{tab:appendix:STAI}
\end{table}

\paragraph{Psychological Outcome Profiles (PSYCHLOPS)}
The PSYCHLOPS \cite{ashworth2004client} consists of four questions. It contains three domains: Problems (2 questions; total score is halved), Function (1 question), and Well-being (1 question). Free text responses are elicited to the Problem and Function domains. Responses are scored on an ordinal six-point scale, producing a maximum score of $18$. The post-therapy version of PSYCHLOPS consists of the same four questions but adds a fifth overall valuation question (determining self-rated outcome ranging from ``much better'' to ``much worse''). \Cref{tab:appendix:PSYCHLOPS} shows the items of the PSYCHLOPS.
\begin{table}[tbh]
    \small
    
    \centering
    \begin{tabular}{m{.06\hsize}m{.81\hsize}}
    \hline
    \textbf{No} & \textbf{PSYCHLOPS Item} \\
    \hline
    1 & Feeling nervous, anxious, or on edge. \\
    2 & Not being able to stop or control worrying. \\
    3 & Worrying too much about different things. \\
    4 & Trouble relaxing. \\
    5 & Being so restless that it is hard to sit still. \\
    6 & Becoming easily annoyed or irritable. \\
    7 & Feeling afraid as if something awful might happen. \\
    \hline
    \end{tabular}
    \caption{Characteristics of the PSYCHLOPS items. Each question starts with ``\textit{Over the last two weeks, how often have you been bothered by any of the following problems?}''}
    \label{tab:appendix:PSYCHLOPS}
\end{table}
